# Supplementary material for: Fundamental Limits on Latency in Transceiver Cache-Aided HetNets
Source: arXiv:1707.09029 source file (2017-07-27)
Supplement: Supplementary file 1 [file appendix_a.tex]

\section{Lower Bounds on DTB (Converse)}
\label{sec:lw_bd}

In this section, we develop lower bounds on the DTB $\Delta_{\text{det}}$ to settle the optimality of our proposed achievability scheme for various regimes of channel parameters $n_{d1},n_{d2}$ and $n_{d3}$. For a given worst-case demand pattern $\mathbf{d}=(d_1, d_2)^{T}$; that is $U_1$ and $U_2$ request \emph{distinct} files $W_{d_1}$ and $W_{d_2}$ ($d_1\neq d_2$), and given channel realization $\mathbf{n}=(n_{d1},n_{d2},n_{d3})^{T}$, we use lower bounds on the delivery time \begin{subequations}
\begin{alignat}{2}
& T_{E} \text{ for } n_{F}=0 \\
& T_{F}+T_{E} \text{ for } n_{F}>0
\end{alignat}
%\begin{equation}\label{eq:time_dur1}
%T_{E} \text{ for } n_{F}=0
%\end{equation}
%\begin{equation}\label{eq:time_dur2}
%T_{F}+T_{E} \text{ for } n_{F}>0
%\end{equation}
\end{subequations}
for the converse on $\Delta_{\text{det}}$. Without loss of generality, we assume that $\mathbf{d}=(1,2)^{T}$, i.e., $W_{d_1}=W_1$ and $W_{d_2}=W_2$. The first bound for (14b) is based on the idea that for any feasible scheme, 
% a (hypothetical) decoder 
$U_1$ or $U_2$ are able to decode $W_1$ and $W_2$ reliably if 
% side information on
they are aware of $\mathbf{S}^{q-\max\{n_{d2},n_{d3}\}}\mathbf{x}_{2}^{T_{E}}$, cached contents $S_1$ and $S_2$ and fronthaul message $\mathbf{S}^{q-n_F}\mathbf{x}_{F}^{T_{F}}$. % are known. 
With knowledge of this % side information, 
collection of information, any decoder can recover $\mathbf{y}_1^{T_E}$ and hence $W_1$ as well as $\mathbf{y}_2^{T_E}$ and thus $W_2$. We obtain the lower bound as follows:   
\begin{eqnarray}\label{eq:conv_1} %\footnotesize
%\arraycolsep=2pt
%\medmuskip = 1mu % default: 4mu plus 2mu minus 4mu
&2L&=H\big(W_1,W_2\big)\nonumber \\& = & I\Big(W_1,W_2;\mathbf{S}^{q-\max\{n_{d2},n_{d3}\}}\mathbf{x}_{2}^{T_{E}},S_1,S_2,\mathbf{S}^{q-n_F}\mathbf{x}_{F}^{T_{F}}\Big)\nonumber \\
 &+&H\big(W_1,W_2|\mathbf{S}^{q-\max\{n_{d2},n_{d3}\}}\mathbf{x}_{2}^{T_{E}},S_1,S_2,\mathbf{S}^{q-n_F}\mathbf{x}_{F}^{T_{F}}\big)\nonumber\\&=& I\Big(W_1,W_2;\mathbf{S}^{q-\max\{n_{d2},n_{d3}\}}\mathbf{x}_{2}^{T_{E}},S_1,S_2,\mathbf{S}^{q-n_F}\mathbf{x}_{F}^{T_{F}}\Big)\nonumber \\
 &+&H\big(W_1|\mathbf{S}^{q-\max\{n_{d2},n_{d3}\}}\mathbf{x}_{2}^{T_{E}},S_1,S_2,\mathbf{S}^{q-n_F}\mathbf{x}_{F}^{T_{F}}\big)\nonumber\\ &+&H\big(W_2|\mathbf{S}^{q-\max\{n_{d2},n_{d3}\}}\mathbf{x}_{2}^{T_{E}},S_1,S_2,\mathbf{S}^{q-n_F}\mathbf{x}_{F}^{T_{F}},W_1\big)\nonumber\\&\stackrel{(a)}\leq& I\Big(W_1,W_2;\mathbf{S}^{q-\max\{n_{d2},n_{d3}\}}\mathbf{x}_{2}^{T_{E}},S_1,S_2,\mathbf{S}^{q-n_F}\mathbf{x}_{F}^{T_{F}}\Big)\nonumber \\ &+&H\big(W_1|\mathbf{S}^{q-\max\{n_{d2},n_{d3}\}}\mathbf{x}_{2}^{T_{E}},S_1,S_2,\mathbf{S}^{q-n_F}\mathbf{x}_{F}^{T_{F}},\mathbf{y}_{1}^{T_{E}}\big)\nonumber\\ &+&H\big(W_2|\mathbf{y}_{2}^{T_{E}},S_1,S_2,\mathbf{S}^{q-n_F}\mathbf{x}_{F}^{T_{F}},W_1,\mathbf{y}_{1}^{T_{E}}\big)\nonumber \\&\stackrel{(b)}\leq & I\Big(W_1,W_2;\mathbf{S}^{q-\max\{n_{d2},n_{d3}\}}\mathbf{x}_{2}^{T_{E}},S_1,S_2,\mathbf{S}^{q-n_F}\mathbf{x}_{F}^{T_{F}}\Big)\nonumber\\&+&L\epsilon_L\nonumber \\ &=& H\Big(\mathbf{S}^{q-\max\{n_{d2},n_{d3}\}}\mathbf{x}_{2}^{T_{E}},S_1,S_2,\mathbf{S}^{q-n_F}\mathbf{x}_{F}^{T_{F}}\Big)+L\epsilon_L\nonumber \\ &\stackrel{(c)}\leq& H\Big(\mathbf{S}^{q-\max\{n_{d2},n_{d3}\}}\mathbf{x}_{2}^{T_{E}}\Big)+H\big(S_1\big)
+H\Big(\mathbf{S}^{q-n_F}\mathbf{x}_{F}^{T_{F}}\Big)\nonumber\\&+& H\Big(S_2,W_2|\mathbf{S}^{q-\max\{n_{d2},n_{d3}\}}\mathbf{x}_{2}^{T_{E}},S_1,\mathbf{S}^{q-n_F}\mathbf{x}_{F}^{T_{F}}\Big)+L\epsilon_L\nonumber\\ &\leq &T_{E}\max\{n_{d2},n_{d3}\}+T_{F}n_{F}+\mu L+L\epsilon_L, \end{eqnarray} 
where (a) is because $\mathbf{y}_{1}^{T_E}$ is a function of $\mathbf{S}^{q-\max\{n_{d2},n_{d3}\}}\mathbf{x}_{2}^{T_{E}}$, $S_1$, $S_2$ and $\mathbf{S}^{q-n_F}\mathbf{x}_{F}^{T_{F}}$ and it is because $\mathbf{S}^{q-\max\{n_{d2},n_{d3}\}}\mathbf{x}_{2}^{T_{E}}$ contains all information on $\mathbf{y}_2^{T_{E}}$, (b) follows from Fano's inequality with $\epsilon_L$ being a term that vanishes as $L\rightarrow\infty$ (c) follows since conditioning does not increase entropy. When rearranging \eqref{eq:conv_1}, we obtain a lower bound on a weighted linear combination of $T_F$ and $T_E$:
\begin{equation}\label{eq:lb_TE_TF}
T_{E}+T_{F}\frac{n_{F}}{\max\{n_{d2},n_{d3}\}}\geq L\Bigg[\frac{2-\mu-\epsilon_L}{\max\{n_{d2},n_{d3}\}}\Bigg].
\end{equation}
%\begin{equation}\label{eq:lb_TE_TF}
%T_{E}\max\{n_{d2},n_{d3}\}+T_{F}n_{F}\geq (2-\mu)L-L\epsilon_L.
%\end{equation}
Finding a lower bound on (14a) follows along the same lines as in \eqref{eq:conv_1} with the difference that the fronthaul link between cloud server and HeNB is not present. This will give us a lower bound solely on $T_E$ as \begin{equation}\label{eq:lb_TE}
T_{E}\geq L\Bigg[\frac{2-\mu-\epsilon_L}{\max\{n_{d2},n_{d3}\}}\Bigg].
\end{equation}
%\begin{equation}\label{eq:lb_TE}
%T_{E}\max\{n_{d2},n_{d3}\}\geq (2-\mu)L-L\epsilon_L.
%\end{equation} 
Since the requested files $W_1$ and $W_2$ can also be retrieved from the received signals $\mathbf{y}_{1}^{T_{E}}$ and $\mathbf{y}_{2}^{T_{E}}$, another lower bound is obtained as follows:
\begin{eqnarray}\label{eq:conv_2} %\footnotesize
%\arraycolsep=2pt
%\medmuskip = 1mu % default: 4mu plus 2mu minus 4mu
&2L&=H\big(W_1,W_2\big)\nonumber \\& = & I\Big(W_1,W_2;\mathbf{y}_{1}^{T_{E}},\mathbf{y}_{2}^{T_{E}}\Big)+H\Big(W_1,W_2|\mathbf{y}_{1}^{T_{E}},\mathbf{y}_{2}^{T_{E}}\Big)\nonumber \\&\stackrel{(a)}\leq& I\Big(W_1,W_2;\mathbf{y}_{1}^{T_{E}},\mathbf{y}_{2}^{T_{E}}\Big)+L\epsilon_L\nonumber\\ % &=&H\big(\mathbf{y}_{1}^{T_{E}},\mathbf{y}_{2}^{T_{E}}\big)\\
&=&H\big(\mathbf{y}_{2}^{T_{E}}\big)+H\big(\mathbf{y}_{1}^{T_{E}}|\mathbf{y}_{2}^{T_{E}}\big)+L\epsilon_L\nonumber\\&=&\sum_{i=1}^{T_E}\Big[H\big(\mathbf{y}_2[i]|\mathbf{y}_2^{i-1}\big)+H\big(\mathbf{y}_1[i]|\mathbf{y}_1^{i-1},\mathbf{y}_2^{T_E}\big)\Big]+L\epsilon_L\nonumber\\&\stackrel{(b)}\leq& \sum_{i=1}^{T_E}\Big[H\big(\mathbf{y}_2[i]\big)+H\big(\mathbf{y}_1[i]|\mathbf{y}_2[i]\big)\Big]+L\epsilon_L\nonumber\\&\stackrel{(c)}\leq& T_{E}n_{d3}+L\epsilon_L\nonumber\\&+&\sum_{i=1}^{T_E}\Big[H\big(\mathbf{S}^{q-n_{d1}}\mathbf{x}_{1}[i]\oplus\mathbf{S}^{q-n_{d2}}\mathbf{x}_{2}[i]|\mathbf{S}^{q-n_{d3}}\mathbf{x}_{2}[i]\big)\Big]\nonumber\\&\stackrel{(d)}\leq&L\epsilon_L+T_{E}\cdot\begin{cases} n_{d1}+n_{d3}&\text{ for } n_{d3}\geq n_{d2} \\ \max\{n_{d1}+n_{d3},n_{d2}\}&\text{ for }n_{d3}\leq n_{d2}
\end{cases}\nonumber\\&=&T_{E}\max\{n_{d1}+n_{d3},n_{d2}\}+L\epsilon_L,\end{eqnarray} 
where (a) follows from Fano's inequality, (b) follows since conditioning does not increase the entropy, (c) is because the $\text{Bern}(\nicefrac{1}{2})$ distribution maximizes the binary entropy of each component of all $n_{d3}$ random elements of $\mathbf{y}_{2}[i]$, (d) follows from the fact that conditioning does not increase entropy and that the randomness in $\mathbf{S}^{q-n_{d2}}\mathbf{x}_{2}[i]$ is fully or partially contained in $\mathbf{S}^{q-n_{d3}}\mathbf{x}_{2}[i]$ depending on whether $n_{d3}\geq n_{d2}$ or $n_{d3}\leq n_{d2}$. Finally, file $W_j$, $j\in\{1,2\}$, must be decodable if $U_{j}$ is aware of $\mathbf{y}_{j}^{T_{E}}$, yielding the lower bound on $T_{E}$ 
\begin{eqnarray}\label{eq:conv_3} %\footnotesize
%\arraycolsep=2pt
%\medmuskip = 1mu % default: 4mu plus 2mu minus 4mu
&L&=H\big(W_j\big)\nonumber \\& = & I\big(W_j;\mathbf{y}_{j}^{T_{E}}\big)+H\big(W_j|\mathbf{y}_{j}^{T_{E}}\big)\nonumber \\&\stackrel{(a)}\leq& I\big(W_j;\mathbf{y}_{j}^{T_{E}}\big)+L\epsilon_L\nonumber\\&\leq& H\big(\mathbf{y}_{j}^{T_{E}}\big)+L\epsilon_{L}\nonumber\\&\leq&L\epsilon_L+T_{E}\cdot\begin{cases}
\max\{n_{d1},n_{d2}\}&\text{ for }j=1\\n_{d3}&\text{ for }j=2\end{cases}, \end{eqnarray} where (a) is due to Fano's inequality.
Rearranging the expressions \eqref{eq:conv_2} and \eqref{eq:conv_3} and letting $L\rightarrow\infty$ such that $\epsilon_L\rightarrow 0$, yields the following lower bound on the DTB:
\begin{equation}\label{eq:dtb_b1}
    \Delta^{*}_{\text{det}}\geq  
  \Delta_{\text{LB}},
\end{equation} where
\begin{equation}\label{eq:dlb}  
  \Delta_{\text{LB}}=\max\Bigg\{\frac{1}{n_{d3}},\frac{1}{\max\{n_{d1},n_{d2}\}}, \frac{2}{\max\{n_{d1}+n_{d3},n_{d2}\}}\Bigg\}
\end{equation}
For the high-fronthaul capacity regime, which we define as $n_F\geq\max\{n_{d2},n_{d3}\}$, we are able to transform the lower bound on the linear combination of $T_F$ and $T_E$ (cf. \eqref{eq:lb_TE_TF}) to a DTB lower bound (applicable for cases where the cloud-to-HeNB fronthaul is active) by combining \eqref{eq:lb_TE_TF} with \eqref{eq:conv_2} and \eqref{eq:conv_3} for $L\rightarrow\infty$. This generates the lower bound 
\begin{equation}\label{eq:dtb_b2}
    \Delta^{*}_{\text{det}}\geq  
  \frac{2-\mu}{n_F}+\Big(1-\frac{\max\{n_{d2},n_{d3}\}}{n_F}\Big)\Delta_{\text{LB}},
\end{equation}
From \eqref{eq:lb_TE}, a lower bound we infer is 
\begin{equation}\label{eq:dtb_b3}
    \Delta^{*}_{\text{det}}\geq  
  \frac{2-\mu}{\max\{n_{d2},n_{d3}\}}.
\end{equation}
We can easily see from \eqref{eq:lb_TE_TF} that \eqref{eq:dtb_b3} functions as a lower bound for $\nicefrac{(T_{E}+F_{F})}{L}$ if we operate in the low-fronthaul capacity regime, which we define as $n_F\leq\max\{n_{d2},n_{d3}\}$.
